# Supplementary material for: Tilt-induced clustering of cell adhesion proteins
Source: arXiv:2307.03670 ancillary file (2023-07-07)
Supplement: Supplementary file 1 [file SI_Lin.pdf]

# Supplemental Material
# Tilt-induced clustering of cell adhesion proteins

Shao-Zhen Lin,[1] Michael P. Sheetz,[2,3] Jacques Prost,[4,2] and Jean-François Rupprecht[1]

[1] *Aix Marseille Univ, Université de Toulon, CNRS, CPT (UMR 7332), Turing Centre for Living systems, Marseille, France*

[2] *Mechanobiology Institute, National University of Singapore, 117411 Singapore*

[3] *Biochemistry and Molecular Biology Department, University of Texas Medical Branch, Galveston, TX 77555*

[4] *Laboratoire Physico-Chimie Curie, UMR 168, Institut Curie, PSL Research University, CNRS, Sorbonne Université, 75005 Paris, France*

(Dated: July 6, 2023)

## CONTENTS

I. Derivation of the entropic contribution 2

II. A simplified microscopic model for the protein tilt optimal angle 2

III. Model details, simulation scheme, and parameter values 3
- A. Governing equations 3
- B. Homogeneous state 4
  - 1. Numerical determination of the homogeneous states 5
  - 2. Analytical expression for the homogeneous states, dilute and dense limits 5
  - 3. Analytical expressions for $h_\phi^{\mathrm{cr},1}$ and $h_\phi^{\mathrm{cr},2}$ 6
  - 4. Analytical expression for $h_\phi^{\mathrm{cr},3}$ 7
- C. Linear stability analysis 8
- D. Link to the Swift–Hohenberg theory 10
- E. Simulation scheme 11
- F. Estimation of parameter values 11

IV. Alternative model with a $\phi$-dependent adhesion stiffness 15

V. Supplemental movies 17

References 17

## I. DERIVATION OF THE ENTROPIC CONTRIBUTION

In [1, 2], adhesion to the glass substrate is mediated though a fixed ligand, composed of a Arginylglycylaspartic acid (RGD) binding site which itself is attached to membrane through biotin through neutravidin molecules.

We assume that the ligands are uniformly distributed, with a typical distance between binders denoted $d$; the typical area of a site is then $a = d^2$.

We consider an elementary patch containing $N \gg 1$ individual ligands. We assume that a number, denoted $N_1$, of those ligands are attached to the cell membrane through a cell adhesion protein, while the remaining ligands are unbound. The number of ways to arrange these $N_1$ proteins among the $N$ available sites is

$$\Omega = \frac{N!}{N_1!(N-N_1)!}. \tag{S1}$$

Within such elementary patch, the configuration entropy density then reads

$$f_{\text{entropy}} = \frac{k_B T}{Na} \ln(\Omega). \tag{S2}$$

In a large number of states limit, the Stirling formula leads us to the expression

$$f_{\text{entropy}} = \frac{k_B T}{a} \left[\phi \ln \phi + (1-\phi) \ln (1-\phi)\right], \tag{S3}$$

where $\phi = N_1/N \in (0,1)$ is the fraction of bound proteins.

In experiments, a typical distance between ligands is typically $d = 10$ nm [1], corresponding to a surface density of $10^4$ molecules/$\mu$m$^2$.

## II. A SIMPLIFIED MICROSCOPIC MODEL FOR THE PROTEIN TILT OPTIMAL ANGLE

Here we provide an expression for the optimal tilt angle based on a microscopic model of adhesion.

We denote by $\theta_i$ the tilt angle of the $i$-th protein. Such tilt angle is defined as the angle between the direction of the protein and the direction of the normal to the membrane (Fig. S1).

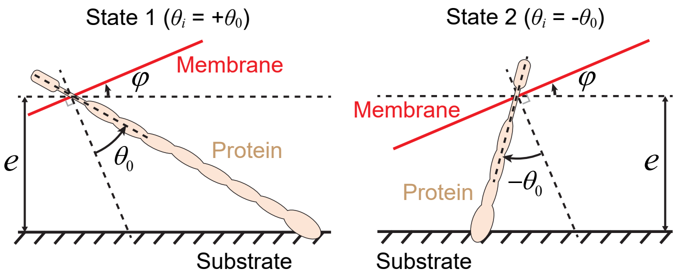


FIG. S1. Sketch of the intrinsic tilt effect of cell adhesion proteins: a two-state microscopic model in 1D to show the symmetry-breaking effect of the protein tilt induced by the membrane height gradient and the flat substrate.

We consider a two-state model in which the protein tilt with respect to the membrane is constrained to take either the following two values: $\theta_i = \pm\theta_0 \neq 0$. Seeing the protein as a rigid rod, such tilt with respect to the membrane results in attached protein being also tilted with respect to the substrate (Fig. S1). A minimal model is to consider that such tilt with respect to the substrate is resisted by a torque, which derives from the following mechanical energy:

$$E_i = \frac{1}{2} K (\theta_i + \varphi)^2, \tag{S4}$$

where $\varphi = \nabla e$ is the angle (along the principal gradient direction of membrane height) due to membrane undulations. Thus, the energy of the state 1 ($\theta_i = +\theta_0$),

$$\text{State 1}: \quad E_+ = \frac{1}{2} K (\theta_0 + \varphi)^2, \tag{S5}$$

and that of the state 2 ($\theta_i = -\theta_0$),

$$\text{State 2}: \quad E_- = \frac{1}{2}K(-\theta_0 + \varphi)^2. \tag{S6}$$

Further assuming Boltzmann statistics in a thermal bath at temperature $T$, the probability of state 1 and state 2 can be expressed by,

$$\text{State 1}: \quad P_+ \sim \frac{1}{Z}\exp\left(-\frac{E_+}{k_B T}\right) = \frac{1}{Z}\exp\left[-\frac{K}{2k_B T}(\theta_0 + \varphi)^2\right], \tag{S7}$$

$$\text{State 2}: \quad P_- \sim \frac{1}{Z}\exp\left(-\frac{E_-}{k_B T}\right) = \frac{1}{Z}\exp\left[-\frac{K}{2k_B T}(-\theta_0 + \varphi)^2\right], \tag{S8}$$

where $Z = \exp(-E_+/k_B T) + \exp(-E_-/k_B T)$ is a renormalization factor, and $k_b$ Boltzmann constant.

In the case of an undulated membrane (i.e. $\varphi = \nabla e \neq 0$), $P_+ \neq P_-$; the appearance probability of state 1 ($\theta_i = +\theta_0$) and state 2 ($\theta_i = -\theta_0$) are unequal. The presence of substrate leads to symmetry breaking of cell adhesion protein tilt angle. The average tilt angle can be further calculated by:

$$\langle\theta_i\rangle = \frac{\theta_0 P_+ - \theta_0 P_-}{P_+ + P_-} = \theta_0 \frac{\exp\left[-\frac{K}{2k_B T}(\theta_0 + \varphi)^2\right] - \exp\left[-\frac{K}{2k_B T}(-\theta_0 + \varphi)^2\right]}{\exp\left[-\frac{K}{2k_B T}(\theta_0 + \varphi)^2\right] + \exp\left[-\frac{K}{2k_B T}(-\theta_0 + \varphi)^2\right]}. \tag{S9}$$

In the limit of a weak effect, $|\varphi| \ll \theta_0$, the mean tilt angle reads

$$\langle\theta_i\rangle \sim -\frac{K\theta_0^2}{k_B T}\varphi = -\frac{K\theta_0^2}{k_B T}\nabla e \neq 0. \tag{S10}$$

In the main text, we defined the average tilt angle minimizing the tilt-induced free energy:

$$\vec{\theta}_{\text{opt}} = -\frac{\mu}{\nu}\vec{\nabla} e. \tag{S11}$$

We identify Eq. (S11) to (S10), such that;

$$\frac{\mu}{\nu} = \frac{K\theta_0^2}{k_B T}. \tag{S12}$$

## III. MODEL DETAILS, SIMULATION SCHEME, AND PARAMETER VALUES

### A. Governing equations

We recall the free energy of the membrane–protein–substrate system considered in the main text:

$$F = \int \mathrm{d}^2\boldsymbol{x} f\left(e; \phi; \nabla e; \nabla^2 e; \nabla\phi\right), \tag{S13}$$

with

$$\begin{aligned} f\left(e; \phi; \nabla e; \nabla^2 e; \nabla\phi\right) = {} & \frac{1}{2}k_0 e^2 - k_0 e_0 (1-\phi)\, e + \frac{1}{2}\kappa\big(\nabla^2 e - c_0\big)^2 + \frac{k_B T}{a}\left[\phi \ln\phi + (1-\phi)\ln(1-\phi)\right] \\ & - h_\phi \phi + \frac{1}{2}D_\phi (\nabla\phi)^2 + \frac{1}{2}(\sigma - \sigma_a \phi)(\nabla e)^2. \end{aligned} \tag{S14}$$

To obtain the minimum energy state of the system, we consider the gradient-descent (frictional) dynamics

$$\frac{\partial e}{\partial t} = -\frac{\delta F}{\delta e} + \eta(\boldsymbol{x}, t), \tag{S15}$$

$$\frac{\partial \phi}{\partial t} = -\frac{\delta F}{\delta \phi}, \tag{S16}$$

where $\eta(\boldsymbol{x},t)$ is the fluctuation, assumed to be Gaussian white noise, satisfying $\langle \eta(\boldsymbol{x},t)\rangle = 0$ and $\langle \eta(\boldsymbol{x},t)\,\eta(\boldsymbol{x}',t')\rangle = \Lambda^2 \delta(\boldsymbol{x}-\boldsymbol{x}')\,\delta(t-t')$ with $\Lambda$ being the noise intensity. Note that for simplicity, we here ignore the fluctuations in $\phi$. Substituting Eq. (S13) into Eqs. (S15) and (S16), we obtain the evolution equations of $e$ and $\phi$ as,

$$\frac{\partial e}{\partial t} = -k_0\left(e - e_0 + e_0\phi\right) - \sigma_a \nabla\phi\cdot\nabla e + \left(\sigma - \sigma_a\phi\right)\nabla^2 e - \kappa\nabla^2\nabla^2 e + \eta(\boldsymbol{x},t)\,, \tag{S17}$$

$$\frac{\partial \phi}{\partial t} = -k_0 e_0 e - \frac{k_B T}{a}\ln\left(\frac{\phi}{1-\phi}\right) + \frac{1}{2}\sigma_a(\nabla e)^2 + h_\phi + D_\phi\nabla^2\phi. \tag{S18}$$

### B. Homogeneous state

Letting $\delta F = 0$, we obtain the steady state of the system which satisfies,

$$\begin{aligned} &k_0\left(e - e_0 + e_0\phi\right) + \kappa\nabla^2\nabla^2 e + \sigma_a\nabla\phi\cdot\nabla e - \left(\sigma - \sigma_a\phi\right)\nabla^2 e = 0,\\ &k_0 e_0 e + \frac{k_B T}{a}\ln\left(\frac{\phi}{1-\phi}\right) - \frac{1}{2}\sigma_a(\nabla e)^2 - h_\phi - D_\phi\nabla^2\phi = 0. \end{aligned} \tag{S19}$$

We further consider the homogeneous state $e(\boldsymbol{x}) = \bar{e}$ and $\phi(\boldsymbol{x}) = \bar{\phi}$. Then Eq. (S19) reduces to

$$\bar{e} = e_0\left(1 - \bar{\phi}\right), \tag{S20}$$

$$-k_0 e_0^2\bar{\phi} + \frac{k_B T}{a}\ln\left(\frac{\bar{\phi}}{1-\bar{\phi}}\right) + k_0 e_0^2 - h_\phi = 0. \tag{S21}$$

We define the function

$$g\left(\bar{\phi}\right) = -k_0 e_0^2\bar{\phi} + \frac{k_B T}{a}\ln\left(\frac{\bar{\phi}}{1-\bar{\phi}}\right) + k_0 e_0^2 - h_\phi. \tag{S22}$$

At edges of the domain, the limit of $g$ are $g\left(\bar{\phi}\to 0\right) = -\infty$ and $g\left(\bar{\phi}\to 1\right) = +\infty$. Therefore, the equation $g(\phi) = 0$ must have real roots in the interval $(0,1)$ and the number of real roots will be odd.

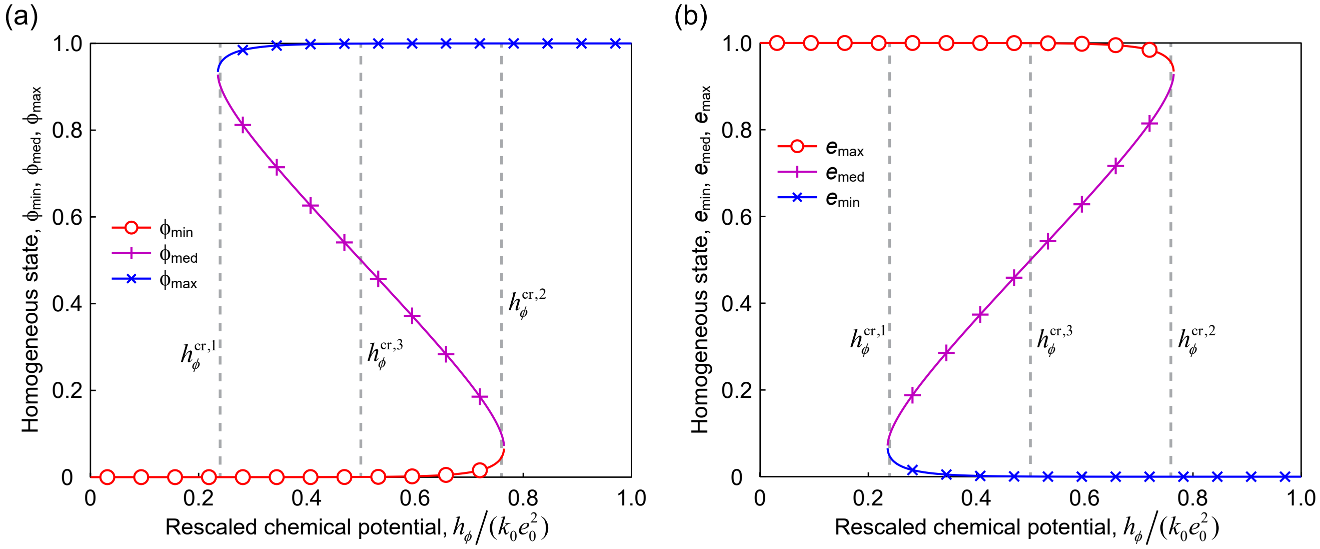


FIG. S2. The homogeneous state $(\bar{e},\bar{\phi})$ as a function of the rescaled chemical potential, $\hat{h}_\phi = h_\phi/(k_0e_0^2)$. (a) $\bar{e}$. (b) $\bar{\phi}$. Here, the solid lines (with symbols) are obtained by directly solving Eqs. (S20) and (S21), using the numerical method described in Sec. III B. The gray dashed lines represent the critical values $h_\phi^{cr,1}$ and $h_\phi^{cr,2}$ (given by Eqs. (S38) and (S39)) and $h_\phi^{cr,3}$ (see Eq. (S41)). See Table S1 for parameter values.

### 1. Numerical determination of the homogeneous states

We next give a numerical approach to solve Eq. (S21) to determine the homogeneous state ($\bar{e}$, $\bar{\phi}$). We first set a seed value $\bar{\phi}$ in the range $(0, 1)$; we then check whether $g(\phi)$ is small enough such that $|g(\phi)| < \varepsilon$ with $\varepsilon = 10^{-8}$ a cutoff threshold.

We show the homogeneous state ($\bar{e}$, $\bar{\phi}$) as a function of the chemical potential $h_\phi$ in Fig. S2. For small values of $h_\phi$, i.e., $h_\phi < h_\phi^{\mathrm{cr},1}$, there exists only one homogeneous state, $\bar{e} \approx e_0$ and $\bar{\phi} \approx 0$, indicating no bound proteins in such a parameter regime. When $h_\phi$ is increased beyond a critical value and below a second critical value, i.e., $h_\phi^{\mathrm{cr},1} < h_\phi < h_\phi^{\mathrm{cr},2}$, there are three homogeneous states, denoted as ($e_{\mathrm{max}}$, $\phi_{\mathrm{min}}$), ($e_{\mathrm{med}}$, $\phi_{\mathrm{med}}$), ($e_{\mathrm{min}}$, $\phi_{\mathrm{max}}$), with $\phi_{\mathrm{min}} \approx 0$ (correspondingly $e_{max} \approx e_0$) and $\phi_{\mathrm{max}} \approx 1$ (correspondingly $e_{\mathrm{min}} \approx 0$). When $h_\phi$ is increased further beyond the second critical value, i.e., $h_\phi > h_\phi^{\mathrm{cr},2}$, again there exists only one homogeneous state, $\bar{e} \approx 0$ and $\bar{\phi} \approx 1$.

In the next subsections, we derive several analytical expressions for the homogeneous states, as well as for the critical chemical potential $h_\phi^{\mathrm{cr},1}$ and $h_\phi^{\mathrm{cr},2}$.

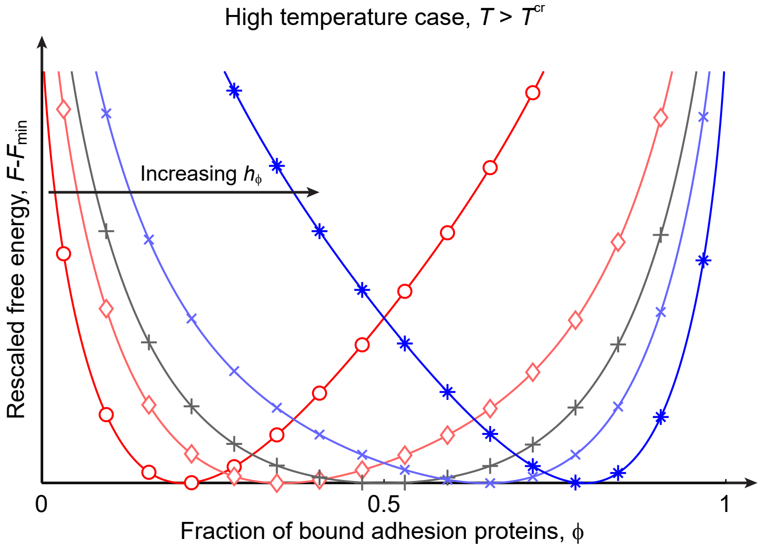


FIG. S3. Sketch of the free energy profiles $F(\phi)$ as a function of $\phi$ at different values of $h_\phi$, for the high temperature case ($T > T^{\mathrm{cr}}$). Here we assume $\phi(\boldsymbol{x}) = \phi$ and $e(\boldsymbol{x}) = e_0(1-\phi)$. $F_{\mathrm{min}} = \min_{\phi\in(0,1)} \{F(\phi)\}$.

### 2. Analytical expression for the homogeneous states, dilute and dense limits

A necessary condition to have only one solution to the condition $g = 0$ is that the derivative of $g$ remains positive. Such derivative reads

$$\frac{\mathrm{d}g}{\mathrm{d}\phi} = -k_0 e_0^2 + \frac{k_B T}{a} \frac{1}{\phi(1-\phi)}. \tag{S23}$$

The minimum of the derivative is

$$\min_{\phi\in(0,1)} \left\{ \frac{\mathrm{d}g}{\mathrm{d}\phi} \right\} = -k_0 e_0^2 + 4\frac{k_B T}{a}. \tag{S24}$$

Such minimum remains positive under the condition

$$-k_0 e_0^2 + 4\frac{k_B T}{a} > 0, \tag{S25}$$

that is,

$$\zeta \triangleq \frac{a k_0 e_0^2}{k_B T} < 4 = \zeta^{\mathrm{cr}}. \tag{S26}$$

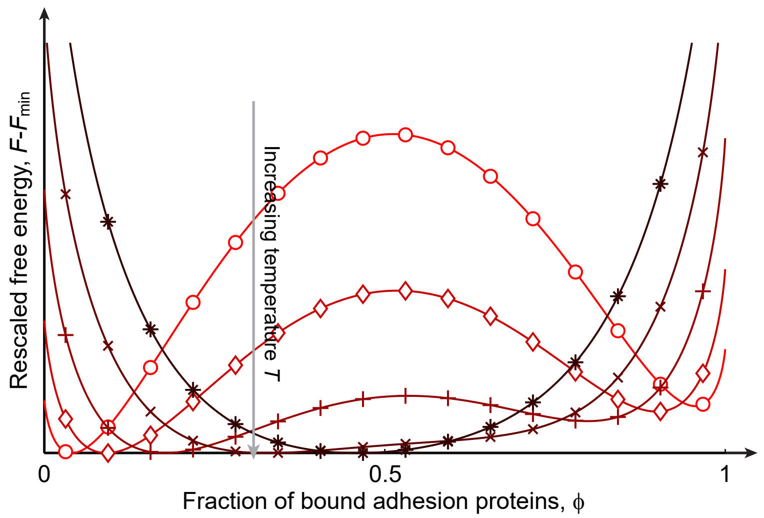


FIG. S4. Sketch of the free energy profiles $F(\phi)$ as a function of $\phi$ at different values of temperature $T$. Here we assume $\phi(\boldsymbol{x}) = \phi$ and $e(\boldsymbol{x}) = e_0(1-\phi)$. $F_{\min} = \min\limits_{\phi\in(0,1)} \{F(\phi)\}$. Here we show the case of $h_\phi < h_\phi^{\mathrm{cr},3}$.

Hence, the latter condition implies that there exists one and only one homogeneous state, regardless of the value of $h_\phi$. Here, $\zeta$ is a non-dimensional parameter that quantifies the ratio of the membrane-substrate repulsion energy ($\sim k_0 e_0^2 a$) to the entropic energy ($\sim k_B T$).

We analyze the behavior of solutions to the equation $g(\phi) = 0$ in the following dilute and dense limits.

- In the dilute phase, i.e., $\bar{\phi} \to 0$, (in which $\bar{e} \to e_0$), we have

$$g\left(\bar{\phi} \to 0\right) \simeq k_0 e_0^2 + \frac{k_B T}{a} \ln \bar{\phi} - h_\phi. \tag{S27}$$

  In such dilute phase limit, the condition $g(\bar{\phi}) = 0$ leads to the following expression

$$\bar{\phi} = \exp\left[\frac{a\left(h_\phi - k_0 e_0^2\right)}{k_B T}\right]. \tag{S28}$$

  Equation (S28) suggests that the existence of a dilute phase $\bar{\phi} \approx 0$ requires that $a(h_\phi - k_0 e_0^2)/k_B T \ll 0$.

- For the dense phase, i.e., $\bar{\phi} \to 1$, (correspondingly $\bar{e} \to 0$), we have

$$g\left(\bar{\phi} \to 1\right) \simeq -\frac{k_B T}{a} \ln\left(1 - \bar{\phi}\right) - h_\phi = 0. \tag{S29}$$

  We thus have the estimation of the dense phase as

$$\bar{\phi} \simeq 1 - \exp\left(-\frac{a h_\phi}{k_B T}\right). \tag{S30}$$

  Equation (S30) suggests that the existence of a dense phase $\bar{\phi} \approx 1$ requires that $h_\phi \gg k_B T/a$.

### *3. Analytical expressions for $h_\phi^{\mathrm{cr},1}$ and $h_\phi^{\mathrm{cr},2}$*

We next obtain the analytical expressions of the critical values $h_\phi^{\mathrm{cr},1}$ and $h_\phi^{\mathrm{cr},2}$. At the critical values $h_\phi = h_\phi^{\mathrm{cr},1}$ or $h_\phi = h_\phi^{\mathrm{cr},2}$, the homogeneous state satisfies Eq. (S21) and $\mathrm{d}g/\mathrm{d}\bar{\phi} = 0$, that is,

$$\zeta\bar{\phi}^2 - \zeta\bar{\phi} + 1 = 0, \tag{S31}$$

where the non-dimensional parameter $\zeta$ is defined in Eq. (S26). Equation (S31) leads to,

$$\bar{\phi} = \frac{1}{2}\left(1 \pm \sqrt{1 - \frac{4}{\zeta}}\right). \tag{S32}$$

The sign $\pm$ in Eq. (S32) corresponds to $h_\phi^{\mathrm{cr},1}$ and $h_\phi^{\mathrm{cr},2}$, respectively. Therefore, we determine the following analytical expressions

$$h_\phi^{\mathrm{cr},1} = k_0 e_0^2 \left[1 - \bar{\phi}_1 + \frac{1}{\zeta} \ln\left(\frac{\bar{\phi}_1}{1 - \bar{\phi}_1}\right)\right], \tag{S33}$$

$$h_\phi^{\mathrm{cr},2} = k_0 e_0^2 \left[1 - \bar{\phi}_2 + \frac{1}{\zeta} \ln\left(\frac{\bar{\phi}_2}{1 - \bar{\phi}_2}\right)\right], \tag{S34}$$

where

$$\bar{\phi}_1 = \frac{1}{2}\left(1 + \sqrt{1 - \frac{4}{\zeta}}\right), \tag{S35}$$

$$\bar{\phi}_2 = \frac{1}{2}\left(1 - \sqrt{1 - \frac{4}{\zeta}}\right). \tag{S36}$$

Since $\bar{\phi}_1$ and $\bar{\phi}_2$ satisfy $\bar{\phi}_1 + \bar{\phi}_2 = 1$ and $\bar{\phi}_1 \bar{\phi}_2 = 1/\zeta$, we find that

$$h_\phi^{\mathrm{cr},1} + h_\phi^{\mathrm{cr},2} = k_0 e_0^2 \left(2 - \bar{\phi}_1 - \bar{\phi}_2\right) + \frac{k_B T}{a} \left\{\ln\left(\bar{\phi}_1 \bar{\phi}_2\right) - \ln\left[\left(1 - \bar{\phi}_1\right)\left(1 - \bar{\phi}_2\right)\right]\right\} = k_0 e_0^2. \tag{S37}$$

Therefore, we have $h_\phi^{\mathrm{cr},1} + h_\phi^{\mathrm{cr},2} = k_0 e_0^2 = 2 h_\phi^{\mathrm{cr},3}$ with $h_\phi^{\mathrm{cr},3}$ being a third critical value (see Eq. (S41)).

Further, in the low temperature limiting case, i.e., $\zeta \gg \zeta_{\mathrm{cr}} = 4$, $\bar{\phi}_1$ and $\bar{\phi}_2$ can be approximated as, $\bar{\phi}_1 \approx 1 - 1/\zeta$ and $\bar{\phi}_2 \approx 1/\zeta$. Thus $h_\phi^{\mathrm{cr},1}$ and $h_\phi^{\mathrm{cr},2}$ can be approximated as,

$$h_\phi^{\mathrm{cr},1} \approx k_0 e_0^2 \left(\frac{1}{\zeta} + \frac{\ln \zeta}{\zeta}\right), \tag{S38}$$

$$h_\phi^{\mathrm{cr},2} \approx k_0 e_0^2 \left(1 - \frac{1}{\zeta} - \frac{\ln \zeta}{\zeta}\right). \tag{S39}$$

In Fig. S2, we show that such approximations agree well with numerical calculations.

### *4. Analytical expression for* $h_\phi^{\mathrm{cr},3}$

In the case of three homogeneous states (i.e., $h_\phi^{\mathrm{cr},1} < h_\phi < h_\phi^{\mathrm{cr},2}$), the free energy density of these three homogeneous states are

$$\begin{aligned} f\left(e_{\max}; \phi_{\min}\right) &\simeq -\frac{1}{2} k_0 e_0^2 \\ f\left(e_{\mathrm{med}}; \phi_{\mathrm{med}}\right) &= -\frac{1}{2} k_0 e_0^2 (1 - \phi_{\mathrm{med}})^2 + \frac{k_B T}{a}\left[\phi_{\mathrm{med}} \ln \phi_{\mathrm{med}} + (1 - \phi_{\mathrm{med}}) \ln\left(1 - \phi_{\mathrm{med}}\right)\right] - h_\phi \phi_{\mathrm{med}} \\ f\left(e_{\min}; \phi_{\max}\right) &\simeq -h_\phi \end{aligned} \tag{S40}$$

Comparing the free energy densities of the homogeneous states $(e_{\max}, \phi_{\min})$ and $(e_{\min}, \phi_{\max})$ leads to a third critical value,

$$h_\phi^{\mathrm{cr},3} = \frac{1}{2} k_0 e_0^2, \tag{S41}$$

such that $f\left(e_{\min}; \phi_{\max}\right) < f\left(e_{\max}; \phi_{\min}\right)$ for $h_\phi^{\mathrm{cr},3} < h_\phi$. We point out that the three critical chemical potentials generally satisfy the inequality:

$$h_\phi^{\mathrm{cr},1} < h_\phi^{\mathrm{cr},3} < h_\phi^{\mathrm{cr},2}, \tag{S42}$$

as illustrated in Fig. S2.

### C. Linear stability analysis

We next consider the stability of the homogeneous state $\left(\bar{e},\bar{\phi}\right)$. The second-order variation of the total free energy $F$ reads,

$$\delta^2 F = \int \mathrm{d}^2\boldsymbol{x}\left\{k_0(\delta e)^2 + \frac{k_B T}{a}\frac{1}{\phi(1-\phi)}(\delta\phi)^2 + (\sigma-\sigma_a\phi)\left[\delta\left(\nabla e\right)\right]^2\right\} + \int \mathrm{d}^2\boldsymbol{x}\left\{\kappa\left[\delta\left(\nabla^2 e\right)\right]^2 + 2k_0 e_0\delta e\delta\phi - 2\sigma_a\nabla e\cdot\delta\phi\delta\left(\nabla e\right) + D_\phi[\delta\left(\nabla\phi\right)]^2\right\}. \tag{S43}$$

At the homogeneous state $(e,\phi)=\left(\bar{e},\bar{\phi}\right)$, such expression reduces to

$$\delta^2 F = \int \mathrm{d}^2\boldsymbol{x}\left\{\begin{aligned}&k_0(\delta e)^2 + \frac{k_B T}{a}\frac{1}{\bar{\phi}(1-\bar{\phi})}(\delta\phi)^2 + \left(\sigma-\sigma_a\bar{\phi}\right)\left[\nabla\left(\delta e\right)\right]^2\\ &+\kappa\left[\nabla^2\left(\delta e\right)\right]^2 + 2k_0 e_0\delta e\delta\phi + D_\phi[\nabla\left(\delta\phi\right)]^2\end{aligned}\right\}. \tag{S44}$$

The latter expression can be re-expressed in the Fourier space as

$$\delta^2 F = \frac{1}{(2\pi)^2}\int \mathrm{d}^2\boldsymbol{q}\left\{\begin{aligned}&\left[k_0 + \left(\sigma-\sigma_a\bar{\phi}\right)|\boldsymbol{q}|^2 + \kappa|\boldsymbol{q}|^4\right]\widetilde{\delta e}\left(\boldsymbol{q}\right)\widetilde{\delta e}\left(-\boldsymbol{q}\right) + k_0 e_0\left[\widetilde{\delta e}\left(\boldsymbol{q}\right)\widetilde{\delta\phi}\left(-\boldsymbol{q}\right) + \widetilde{\delta e}\left(-\boldsymbol{q}\right)\widetilde{\delta\phi}\left(\boldsymbol{q}\right)\right]\\ &+\left[\frac{k_B T}{a}\frac{1}{\bar{\phi}(1-\bar{\phi})} + D_\phi|\boldsymbol{q}|^2\right]\widetilde{\delta\phi}\left(\boldsymbol{q}\right)\widetilde{\delta\phi}\left(-\boldsymbol{q}\right)\end{aligned}\right\}, \tag{S45}$$

where $\widetilde{\delta e}\left(\boldsymbol{q}\right)=\int \mathrm{d}^2\boldsymbol{q}\delta e\left(\boldsymbol{x}\right)\exp\left(-\mathrm{i}\boldsymbol{q}\cdot\boldsymbol{x}\right)$ and $\widetilde{\delta\phi}\left(\boldsymbol{q}\right)=\int \mathrm{d}^2\boldsymbol{q}\delta\phi\left(\boldsymbol{x}\right)\exp\left(-\mathrm{i}\boldsymbol{q}\cdot\boldsymbol{x}\right)$ are the Fourier transforms of $\delta e$ and $\delta\phi$, respectively. Further, letting

$$\boldsymbol{\Phi}\left(\boldsymbol{q}\right) = \begin{pmatrix}\widehat{\widetilde{\delta e}}\left(\boldsymbol{q}\right)\\ \widehat{\widetilde{\delta\phi}}\left(\boldsymbol{q}\right)\end{pmatrix}, \tag{S46}$$

and

$$\boldsymbol{J}\left(\boldsymbol{q}\right) = \begin{pmatrix}k_0 e_0^2 + \left(\sigma-\sigma_a\bar{\phi}\right)e_0^2|\boldsymbol{q}|^2 + \kappa e_0^2|\boldsymbol{q}|^4 & k_0 e_0^2\\ k_0 e_0^2 & \dfrac{k_B T}{a}\dfrac{1}{\bar{\phi}(1-\bar{\phi})} + D_\phi|\boldsymbol{q}|^2\end{pmatrix}, \tag{S47}$$

with $\widehat{\widetilde{\delta e}}=\widetilde{\delta e}/e_0$ and $\widehat{\widetilde{\delta\phi}}=\widetilde{\delta\phi}$ being the rescaled $\widetilde{\delta e}$ and $\widetilde{\delta\phi}$. Eq. (S45) can be re-expressed as

$$\delta^2 F = \frac{1}{(2\pi)^2}\int \mathrm{d}^2\boldsymbol{q}\hat{\boldsymbol{\Phi}}\left(\boldsymbol{q}\right)\cdot\boldsymbol{J}\left(\boldsymbol{q}\right)\cdot\boldsymbol{\Phi}\left(\boldsymbol{q}\right), \tag{S48}$$

where $\hat{\boldsymbol{\Phi}}\left(\boldsymbol{q}\right)=\boldsymbol{\Phi}\left(-\boldsymbol{q}\right)$ is the conjugate complex of $\boldsymbol{\Phi}\left(\boldsymbol{q}\right)$. Therefore, the Jacobian matrix $\boldsymbol{J}\left(\boldsymbol{q}\right)$ determines the stability of the homogeneous state $(e,\phi)=\left(\bar{e},\bar{\phi}\right)$.

We next seek to solve the eigenvalues of $\boldsymbol{J}\left(\boldsymbol{q}\right)$. Denote them as $\lambda\left(\boldsymbol{q}\right)=\lambda\left(|\boldsymbol{q}|\right)=\lambda\left(q\right)$ with $q=|\boldsymbol{q}|$. The characteristic equation reads

$$\lambda^2 - \alpha\lambda + \beta = 0, \tag{S49}$$

where the coefficients $\alpha$ and $\beta$ are

$$\begin{aligned}\alpha &= \kappa e_0^2 q^4 + \left(\sigma e_0^2 - \sigma_a e_0^2\bar{\phi} + D_\phi\right)q^2 + k_0 e_0^2 + \frac{k_B T}{a}\frac{1}{\bar{\phi}(1-\bar{\phi})},\\ \beta &= \left[k_0 e_0^2 + \left(\sigma-\sigma_a\bar{\phi}\right)e_0^2 q^2 + \kappa e_0^2 q^4\right]\left[\frac{k_B T}{a}\frac{1}{\bar{\phi}(1-\bar{\phi})} + D_\phi q^2\right] - k_0^2 e_0^4.\end{aligned} \tag{S50}$$

Therefore the eigenvalues of $\boldsymbol{J}\left(\boldsymbol{q}\right)$ are

$$\lambda = \frac{\alpha\pm\sqrt{\alpha^2-4\beta}}{2} \quad\Rightarrow\quad \lambda_+ = \frac{\alpha+\sqrt{\alpha^2-4\beta}}{2},\ \lambda_- = \frac{\alpha-\sqrt{\alpha^2-4\beta}}{2} \tag{S51}$$

Note that $\alpha^2 - 4\beta > 0$ holds for arbitrary parameters and all $q > 0$. The stability condition of the homogeneous state $(e, \phi) = (\bar{e}, \bar{\phi})$ is

$$\lambda_- = \frac{\alpha - \sqrt{\alpha^2 - 4\beta}}{2} > 0 \quad (\forall q) \qquad \Leftrightarrow \qquad \alpha > 0 \ , \ \beta > 0 \quad (\forall q) \tag{S52}$$

We find that $\beta > 0$ implies that $\alpha > 0$. Indeed, we show that

$$\begin{aligned} &\beta = \left[k_0 e_0^2 + \left(\sigma - \sigma_a \bar{\phi}\right) e_0^2 q^2 + \kappa e_0^2 q^4\right] \left[\frac{k_B T}{a} \frac{1}{\bar{\phi}(1-\bar{\phi})} + D_\phi q^2\right] - k_0^2 e_0^4 > 0 \\ &\Rightarrow \left[k_0 e_0^2 + \left(\sigma - \sigma_a \bar{\phi}\right) e_0^2 q^2 + \kappa e_0^2 q^4\right] \left[\frac{k_B T}{a} \frac{1}{\bar{\phi}(1-\bar{\phi})} + D_\phi q^2\right] > k_0^2 e_0^4 > 0 \\ &\Rightarrow k_0 e_0^2 + \left(\sigma - \sigma_a \bar{\phi}\right) e_0^2 q^2 + \kappa e_0^2 q^4 > 0 \\ &\Rightarrow \alpha = \left[k_0 e_0^2 + \left(\sigma - \sigma_a \bar{\phi}\right) e_0^2 q^2 + \kappa e_0^2 q^4\right] + \left[\frac{k_B T}{a} \frac{1}{\bar{\phi}(1-\bar{\phi})} + D_\phi q^2\right] > 0 \end{aligned} \tag{S53}$$

Thus once $\beta > 0$, $\alpha > 0$ is automatically satisfied. Therefore, the stability condition requires

$$\beta > 0 \quad (\forall q)\,. \tag{S54}$$

We analyze the behavior of the function $\beta$ in the following dilute and dense limits.

- We first consider the dilute homogeneous state $(e_{\max},\, \phi_{\min})$. Since $\phi_{\min} \approx 0$ (Fig. S2), we have

$$\alpha(\phi_{\min}) \simeq \frac{k_B T}{a} \frac{1}{\phi_{\min}} \gg 0, \tag{S55}$$

$$\beta(\phi_{\min}) \simeq \frac{k_B T}{a} \frac{1}{\phi_{\min}} \left(\kappa e_0^2 q^4 + \sigma e_0^2 q^2 + k_0 e_0^2\right) \simeq \alpha(\phi_{\min}) \left(\kappa e_0^2 q^4 + \sigma e_0^2 q^2 + k_0 e_0^2\right) \gg 0, \tag{S56}$$

  which together result in the eigenvalue

$$\lambda_-(\phi_{\min}) = \frac{\alpha - \sqrt{\alpha^2 - 4\beta}}{2} = \frac{2\beta}{\left(\alpha + \sqrt{\alpha^2 - 4\beta}\right)} \simeq \frac{\beta}{\alpha} \simeq \kappa e_0^2 q^4 + \sigma e_0^2 q^2 + k_0 e_0^2 > 0. \tag{S57}$$

  This suggests that the homogeneous state $(e_{\max},\, \phi_{\min})$ is always stable.

- We now consider the homogeneous state $(e_{\min},\, \phi_{\max})$. Since $\phi_{\max} \approx 1$ (Fig. S2), we have

$$\alpha(\phi_{\max}) \simeq \frac{k_B T}{a} \frac{1}{1 - \phi_{\max}} \gg 0, \tag{S58}$$

$$\beta(\phi_{\max}) \simeq \frac{k_B T}{a} \frac{1}{1 - \phi_{\max}} \left[\kappa e_0^2 q^4 + (\sigma - \sigma_a)\, e_0^2 q^2 + k_0 e_0^2\right] \simeq \alpha(\phi_{\max}) \left[\kappa e_0^2 q^4 + (\sigma - \sigma_a)\, e_0^2 q^2 + k_0 e_0^2\right], \tag{S59}$$

  which leads to the eigenvalue as

$$\lambda_-(\phi_{\max}) = \frac{\alpha - \sqrt{\alpha^2 - 4\beta}}{2} = \frac{2\beta}{\left(\alpha + \sqrt{\alpha^2 - 4\beta}\right)} \simeq \frac{\beta}{\alpha} \simeq \kappa e_0^2 q^4 + (\sigma - \sigma_a)\, e_0^2 q^2 + k_0 e_0^2. \tag{S60}$$

  Consequently, minimizing $\lambda_-$ over wavenumbers $q$, we obtain

$$\min_q \{\lambda_-\} \simeq \begin{cases} k_0 & , \quad \sigma_a < \sigma \\ k_0 - \dfrac{(\sigma - \sigma_a)^2}{4\kappa} & , \quad \sigma_a > \sigma \end{cases} \tag{S61}$$

which leads to a critical value of $\sigma_a$ as,

$$\sigma_a^{\rm cr} = \sigma + 2\sqrt{k_0\kappa}. \tag{S62}$$

When $\sigma_a > \sigma_a^{\rm cr}$, the homogeneous state ($e_{\rm min}$, $\phi_{\rm max}$) becomes unstable. The most unstable mode is

$$q_{\rm min} = \sqrt{\frac{\sigma_a - \sigma}{2\kappa}}, \tag{S63}$$

which corresponds to a typical cluster size

$$\xi = \frac{2\pi}{q_{\rm min}} = 2\pi\sqrt{\frac{2\kappa}{\sigma_a - \sigma}}. \tag{S64}$$

At the critical point $\sigma_a = \sigma_a^{\rm cr}$, Eq. (S64) reads

$$\xi^{\rm cr} = 2\pi\sqrt{\frac{2\kappa}{\sigma_a^{\rm cr} - \sigma}} = 2\pi\left(\frac{\kappa}{k_0}\right)^{\frac{1}{4}}. \tag{S65}$$

This gives an upper bound of cluster size. Our numerical simulations validate such a power-law scaling behavior of the cluster size, see Fig. S5.

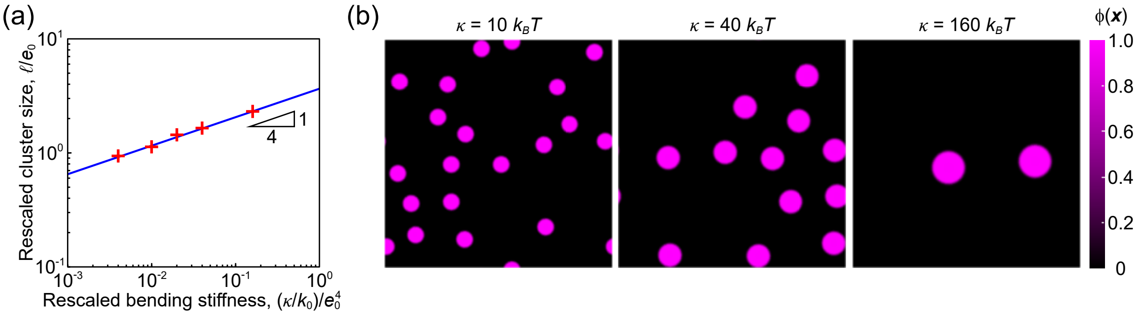


FIG. S5. The cell adhesion proteins cluster size $\ell$ depends on the membrane bending stiffness $\kappa$ and the membrane-substrate adhesion stiffness $k_0$. (a) The cluster size $\ell$ scales in a power-law behavior with the membrane bending stiffness $\kappa$ and the membrane-substrate adhesion stiffness $k_0$ as, $\ell \propto (\kappa/k_0)^{1/4}$. Symbols represent data obtained from numerical simulations where we vary the values of $\kappa$ and $\sigma_a$ while keeping $\hat{\sigma}_a = (\sigma_a - \sigma)/\sqrt{k_0\kappa}$ constant. (b) Typical patterns of bound cell adhesion proteins at different values of $\kappa$ while keeping $\hat{\sigma}_a = (\sigma_a - \sigma)/\sqrt{k_0\kappa}$ constant. Simulation domain size $= L \times L$ with $L = 16e_0 = 1280$ nm. Parameters: $\hat{\sigma}_a = (\sigma_a - \sigma)/\sqrt{k_0\kappa} = 3.4$ and $\hat{h}_\phi = h_\phi/(k_0 e_0^2) = 0.3$; see Table S1 for other parameter values.

## D. Link to the Swift–Hohenberg theory

Our numerical simulations show the existence of circular clustering of hexagon-like patterns and line-structured patterns. This is reminiscent of the pattern formation in the Swift–Hohenberg theory [3, 4]. To better illustrate the connection of our theory to the Swift–Hohenberg theory, we here focus on a simple case where we impose $e = e_0(1-\phi)$, as indicated by the homogeneous state equation (S20). In such a simplified case, the free energy density Eq. (S14) reduces to,

$$f\left(\phi; \nabla\phi; \nabla^2\phi\right) = -\frac{1}{2}k_0 e_0^2 (1-\phi)^2 + \frac{1}{2}\kappa e_0^2\left(\nabla^2\phi + \frac{c_0}{e_0}\right)^2 + \frac{k_B T}{a}\left[\phi\ln\phi + (1-\phi)\ln(1-\phi)\right] - h_\phi\phi + \frac{1}{2}\left(D_\phi + \sigma e_0^2 - \sigma_a e_0^2\phi\right)(\nabla\phi)^2. \tag{S66}$$

We then find that the dynamic evolution equation of $\phi$, $\partial\phi/\partial t = -\delta F/\delta\phi$, can be expressed as

$$\frac{\partial\phi}{\partial t} = k_0 e_0^2\phi - \left(\sigma_a e_0^2\phi - \sigma e_0^2 - D_\phi\right)\nabla^2\phi - \kappa e_0^2\nabla^2\nabla^2\phi - \frac{k_B T}{a}\ln\left(\frac{\phi}{1-\phi}\right) + h_\phi - k_0 e_0^2 - \frac{1}{2}\sigma_a e_0^2(\nabla\phi)^2. \tag{S67}$$

In the regime $\sigma_a > \sigma_a^{\text{cr}}$ (such that $\sigma_a e_0^2 \phi - \sigma e_0^2 - D_\phi > 0$), and Eq. (S67) can be recast as a Swift–Hohenberg like equation (rescaling time in units of $\kappa e_0^2$),

$$\frac{\partial \phi}{\partial t} = \left[\mu - \left(q_c^2(\phi) + \nabla^2\right)^2\right] \phi + m\left(\phi\right), \tag{S68}$$

with

$$q_c^2(\phi) = \frac{\sigma_a e_0^2 \phi - \sigma e_0^2 - D_\phi}{2\kappa e_0^2}, \tag{S69}$$

$$\mu = q_c^4(\phi) + \frac{k_0}{\kappa}, \tag{S70}$$

$$m(\phi) = \frac{h_\phi - k_0 e_0^2}{\kappa e_0^2} - \frac{k_B T}{a\kappa e_0^2} \ln\left(\frac{\phi}{1-\phi}\right) - \frac{\sigma_a e_0^2}{2\kappa e_0^2} \left(\nabla \phi\right)^2. \tag{S71}$$

The non-linear $m(\phi)$ expression contains a quadratic contribution in $\phi$, which is known to favor the formation of a hexagon pattern of circular patches [4].

### E. Simulation scheme

*Simulation method* We use the spectral method to solve the controlling equations (S17) and (S18). The time integration is performed using a backward Euler scheme; the spatial derivatives are carried out using a second-order central difference method. Simulations were performed on a $256 \times 256$ two-dimensional lattice using periodic boundary conditions.

*Annealing procedure* To converge to the energy minimum, we consider the following gradient-descent dynamics, $\dot{\phi} = -\delta F/\delta\phi$, and $\dot{e} = -\delta F/\delta e + \eta(x,t)$; the white noise is discretized as,

$$\eta\left(\boldsymbol{x}, t\right) = \frac{\Lambda}{\sqrt{\left(\Delta x\right)^2 \Delta t}} \vartheta, \tag{S72}$$

where $\vartheta$ is the normal distribution, generated by the built-in function "randn" in MATLAB [5]. To approach the global energy minimum state, we performed annealing simulations where we decrease the noise intensity $\Lambda$ gradually from $\Lambda = 10$ to $\Lambda = 0$. We set the initial $e$ field and $\phi$ field as uniform $(e_{\text{med}}, \phi_{\text{med}})$ but with small perturbations. We decrease $\Lambda$ quasi-statically, according to the iterative process:

1. relaxing the system to reach a steady state with a noise level $\Lambda^{(0)} = 10$,

2. reduce the noise intensity to $\Lambda^{(i+1)} = \Lambda^{(i)} + \Delta\Lambda$ with $\Delta\Lambda = -0.1$.

We repeat the above two steps until $\Lambda = 0$.

*Initialization* The initial condition for the fields $e$ and $\phi$ is a homogeneous steady state (either $(e_{\text{med}}, \phi_{\text{med}})$ for $T < T^{\text{cr}}$, or the only homogeneous state otherwise $T > T^{\text{cr}}$), with small perturbations, $e(\boldsymbol{x}, t=0) = e_{\text{med}} + \varepsilon_e \vartheta_e(\boldsymbol{x})$ and $\phi(\boldsymbol{x}, t=0) = \phi_{\text{med}} + \varepsilon_\phi \vartheta_\phi(\boldsymbol{x})$, where $\varepsilon_e = 10^{-3}$ and $\varepsilon_\phi = 10^{-3}$; $\vartheta_e(\boldsymbol{x})$ and $\vartheta_\phi(\boldsymbol{x})$ are random valuables satisfying the normal distribution.

We checked to start with a different initial condition (e.g. with random perturbations to the homogeneous steady state $(e_{\max}, \phi_{\min})$ or $(e_{\min}, \phi_{\max})$ in the low temperature case $T < T^{\text{cr}}$). We find that the final clustering pattern at $\Lambda = 0$ does not depend on the initial states.

### F. Estimation of parameter values

*Surface tension* Previous studies reported that the cell membrane surface tension $\sigma$ is $\sim 10^{-5}$ J $\cdot$ m$^{-2}$ [6–8]. In our study here we take a value of $\sigma = 2 \times 10^{-5}$ J $\cdot$ m$^{-2} \simeq 0.005\ k_B T \cdot$ nm$^{-2}$.

*Membrane-substrate adhesion stiffness* $k_0$ Assuming the area ($a$) and the adhesion energy ($\sim k_0 e_0^2 a$) of a single cell adhesion protein molecule to be $a = 100$ nm$^2$ and $k_0 e_0^2 a \sim 10 k_B T$, respectively, we can estimate the membrane-substrate binding stiffness as, $k_0 \sim 10 k_B T/(e_0^2 a) \sim 10^{11}$ J $\cdot$ m$^{-4}$. Correspondingly, the adhesion strength can be roughly estimated by, $\lambda \sim k_0 a \sim 10^{-3}$ $k_B T \cdot$ nm$^{-2}$, which is consistent with that assumed in Ref. [9]. In our simulations we set $k_0 = 10^{11}$ J $\cdot$ m$^{-4} \approx 2.5 \times 10^{-5} k_B T \cdot$ nm$^{-4}$.

According to previous studies, unless stated otherwise, we use the parameter values as described in Table S1. In our simulations, we normalize the parameters by the length scale $e_0 = 80$ nm [9–11] and the energy scale $k_B T = 4 \times 10^{-21}$J. We set the non-dimensional parameters as below: $\tilde{k}_0 = k_0 e_0^4/(k_B T) = 1000$, $\tilde{\kappa} = \kappa/(k_B T) = 10$, $\tilde{\sigma} = \sigma e_0^2/(k_B T) = 32$, $\tilde{a} = a/e_0^2 = 1/64$, $\tilde{D}_\phi = D_\phi/(k_B T) = 1$.

TABLE S1. List of default parameter values used in our simulation

| Parameter | Description | Value (dimensionless) | Value (dimension) |
|---|---|---|---|
| $\ell = e_0$ | Length scale | 1 | 80 nm [9–11] |
| $w = k_B T$ | Energy scale | 1 | $4 \times 10^{-21}$ J |
| $k_0$ | Membrane-substrate adhesion stiffness | 1000 | $10^{11}$ J $\cdot$ m$^{-4}$ [9, 11] |
| $\kappa$ | Cell membrane bending stiffness | 10 | $4 \times 10^{-20}$ J [8, 9, 11–13] |
| $\sigma$ | Cell membrane surface tension | 32 | $2 \times 10^{-5}$ J $\cdot$ m$^{-2}$ [6–8] |
| $a$ | Inverse areal density of binders | 1/64 | $10^{-16}$ m$^2$ [8, 14] |
| $D_\phi$ | Gradient energy coefficient | 1 | $4 \times 10^{-21}$ J |
| $h_\phi^{\mathrm{cr},1}$ | First critical value of $h_\phi$ | 235.6 | $1.513 \times 10^{-4}$ J $\cdot$ m$^{-2}$ |
| $h_\phi^{\mathrm{cr},2}$ | Second critical value of $h_\phi$ | 764.4 | $4.909 \times 10^{-4}$ J $\cdot$ m$^{-2}$ |
| $h_\phi^{\mathrm{cr},3}$ | Third critical value of $h_\phi$ | 500 | $3.211 \times 10^{-4}$ J $\cdot$ m$^{-2}$ |
| $\Delta x$ | Lattice mesh size | 1/16 | 5 nm |
| $\Delta t$ | Gradient-descent time step | $10^{-6}$ | — |

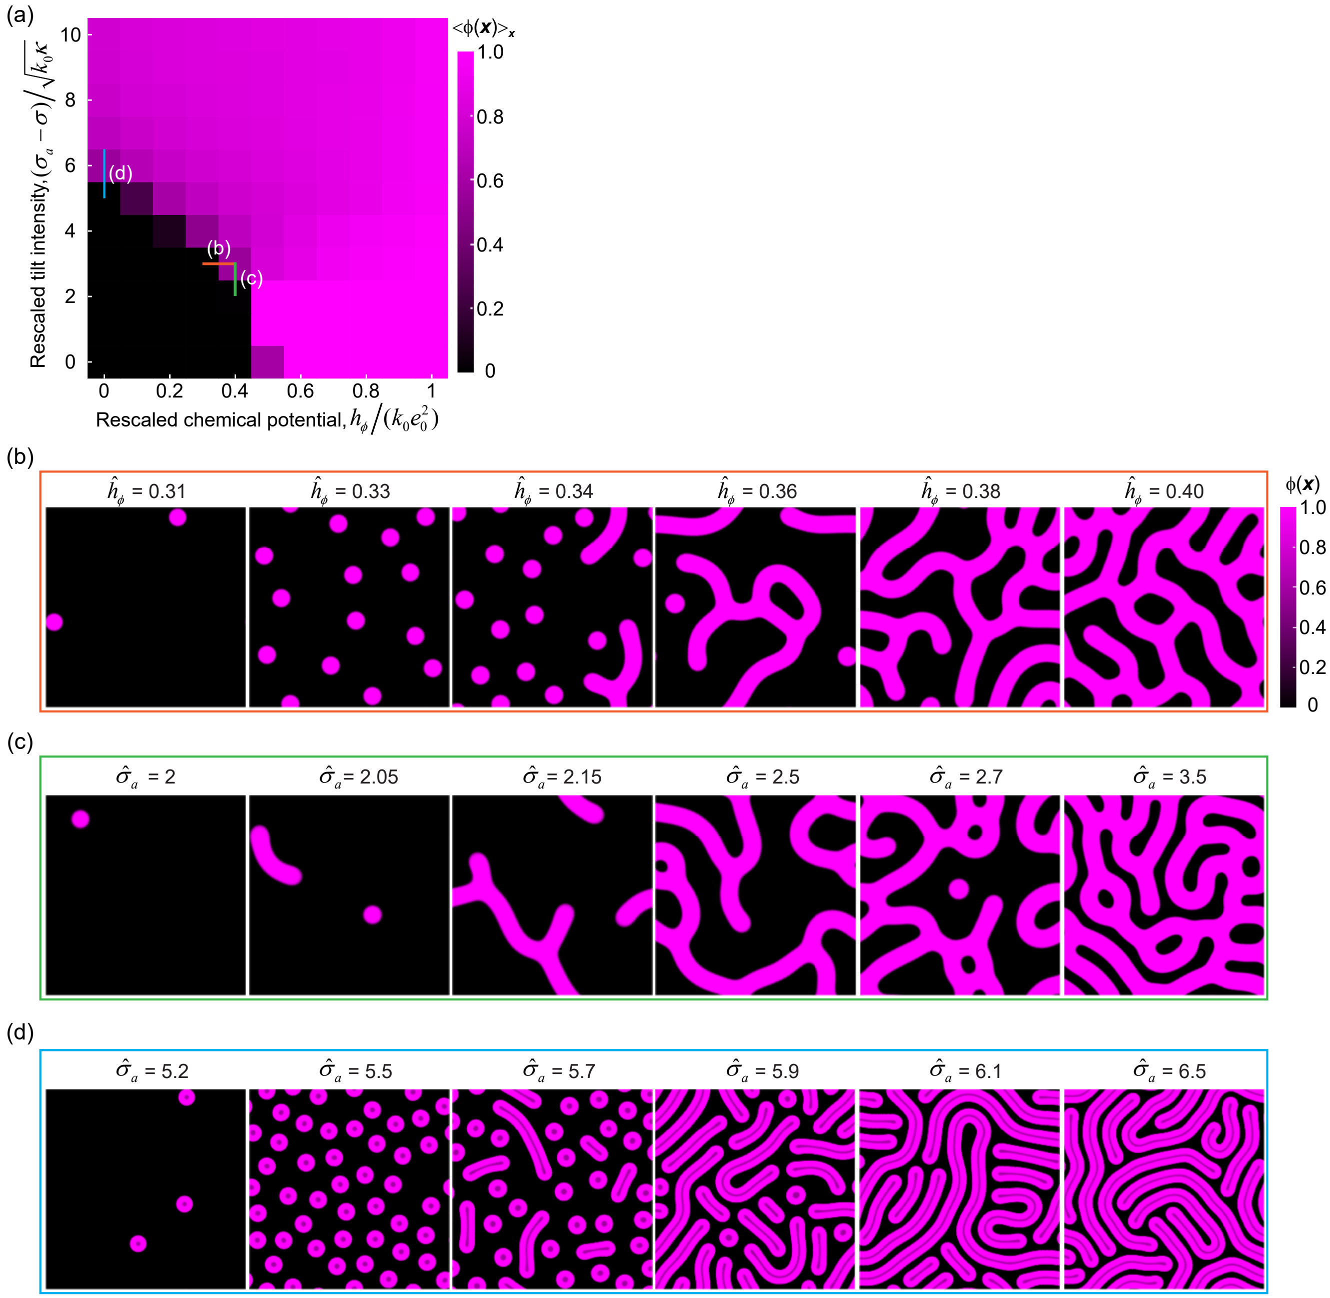


FIG. S6. (a) Diagram of the fraction of bound cell adhesion proteins averaged over the whole space (dark, $\langle\phi\rangle = 0$; light magenta, $\langle\phi\rangle = 1$), as a function on the rescaled chemical potential, $h_\phi/(k_0 e_0^2)$, and the rescaled intensity of protein tilt effect, $(\sigma_a - \sigma)/\sqrt{k_0\kappa}$. (b) Typical patterns of bound cell adhesion proteins at different values of $\hat{h}_\phi = h_\phi/(k_0 e_0^2)$ (see the orange line in (a)), where $\hat{\sigma}_a = (\sigma_a - \sigma)/\sqrt{k_0\kappa} = 3$. (c, d) Typical patterns of bound cell adhesion proteins at different values of $\sigma_a$ (see the green line and the cyan line in (a)), where $\hat{h}_\phi = h_\phi/(k_0 e_0^2) = 0.4$ in (c) and $\hat{h}_\phi = h_\phi/(k_0 e_0^2) = 0$ in (d). In (b-d), simulation domain size $= L \times L$ with $L = 16e_0 = 1280$ nm. See Table S1 for other parameter values.

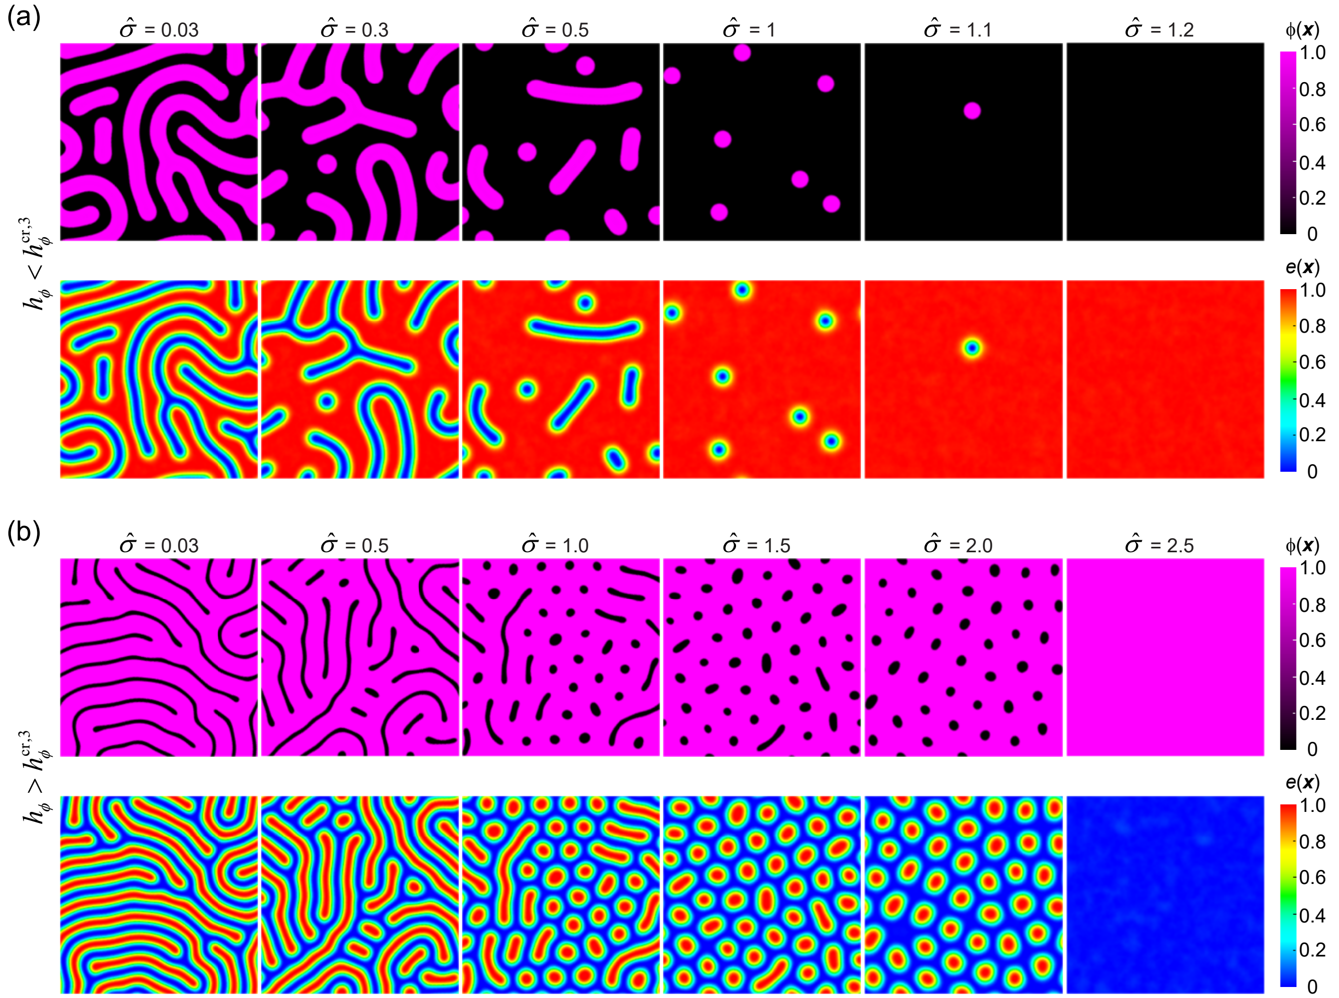


FIG. S7. Depending on the value of $h_\phi$ with respect to $h^{\mathrm{cr},3}$, an increase in the membrane tension $\sigma$ can either lead to a fully dilute state in the case of $h_\phi < h_\phi^{\mathrm{cr},3}$, or to a fully dense state in the case of $h_\phi > h_\phi^{\mathrm{cr},3}$. (a) In the case of $h_\phi < h_\phi^{\mathrm{cr},3}$, an increase in the membrane tension $\sigma$ leads to the disappearance of adhesion clusters. The rescaled membrane tension is defined as, $\hat{\sigma} = \sigma/\sqrt{k_0\kappa}$. Top: the $\phi(\boldsymbol{x})$ field; bottom: the $e(\boldsymbol{x})$ field. Parameters: $\hat{h}_\phi = h_\phi/(k_0 e_0^2) = 0.3$ and $\hat{\sigma}_a = \sigma_a/\sqrt{k_0\kappa} = 4$. (b) In the case of $h_\phi > h_\phi^{\mathrm{cr},3}$, an increase in the membrane tension $\sigma$ leads to a fully dense state. Simulation domain size $= L \times L$ with $L = 16e_0 = 1280$ nm. Parameters: $\hat{h}_\phi = h_\phi/(k_0 e_0^2) = 0.6$ and $\hat{\sigma}_a = \sigma_a/\sqrt{k_0\kappa} = 5$. See Table S1 for other parameter values.

## IV. ALTERNATIVE MODEL WITH A $\phi$-DEPENDENT ADHESION STIFFNESS

Up to now (as well as in the main text), we focused on the case of a membrane-substrate adhesion energy, $F_{\text{adh}}$ with a constant adhesion stiffness, $k(\phi) = k_0$.

However, experiments reviewed in [9] have suggested that the membrane stiffness is significantly weaker in the absence of cell adhesion proteins; typically, $k_0(\phi = 0) \sim \gamma \sim 10^{-7} k_B T \cdot \text{nm}^{-4}$ (following the value for $\gamma$ provided in [9]) instead of $k_0(\phi = 1) \sim \lambda/a \sim 10^{-4} k_B T \cdot \text{nm}^{-4}$ for fully adhered membranes (with $a = 100\ \text{nm}^2$, and using the value $\lambda = 10^{-2} k_B T \cdot \text{nm}^{-2}$ [9]).

Nevertheless, here we show that considering an explicit dependence of $k_0$ on $\phi$ does not change the overall phenomenology.

We propose an alternative free energy of the membrane-substrate adhesion where we include another membrane-substrate adhesion elasticity and its adhesion stiffness $k_1(\phi)$ depends on $\phi$,

$$F_{\text{adh}} = \int \mathrm{d}^2\boldsymbol{x} \left\{ \frac{1}{2} k_0 (e - e_0)^2 + \frac{1}{2} k_1(\phi)(e - e_1)^2 - h_\phi \phi \right\}. \tag{S73}$$

Here $e_1$ is the membrane-substrate distance when the cell adhesion proteins fully bind to the substrate; $k_1(\phi)$ describes the enforcement effect of bound proteins on membrane-substrate adhesion, thus increasing with increasing $\phi$. Assuming a linear dependence of $k_1(\phi)$ on $\phi$, i.e., $k_1(\phi) = k_1\phi$, the adhesion energy then reads,

$$\begin{aligned} F_{\text{adh}} &= \int \mathrm{d}^2\boldsymbol{x} \left\{ \frac{1}{2} k_0 (e - e_0)^2 + \frac{1}{2} k_1 \phi (e - e_1)^2 - h_\phi \phi \right\} \\ &= \int \mathrm{d}^2\boldsymbol{x} \left\{ \frac{1}{2} \left(k_0 + k_1\phi\right) e^2 - \left(k_0 e_0 + k_1 e_1 \phi\right) e - \left( h_\phi - \frac{1}{2} k_1 e_1^2 \right) \phi + \frac{1}{2} k_0 e_0^2 \right\}, \end{aligned} \tag{S74}$$

that is,

$$F_{\text{adh}} = \int \mathrm{d}^2\boldsymbol{x} \left\{ \frac{1}{2} k\left(\phi\right) e^2 - k\left(\phi\right) e_0\left(\phi\right) e - \hat{h}_\phi \phi + \frac{1}{2} k_0 e_0^2 \right\}, \tag{S75}$$

where $\hat{h}_\phi = h_\phi - k_1 e_1^2/2$; the $\phi$-dependent stiffness $k(\phi)$ and preferred distance $e_0(\phi)$ are,

$$k\left(\phi\right) = k_0 + k_1 \phi \quad , \quad e_0\left(\phi\right) = \frac{k_0 e_0 + k_1 e_1 \phi}{k_0 + k_1 \phi}. \tag{S76}$$

Correspondingly, the total free energy of the cell membrane–protein–substrate system now reads

$$F = \int \mathrm{d}^2\boldsymbol{x} \left\{ \begin{aligned} &\frac{1}{2} k_0 (e - e_0)^2 + \frac{1}{2} k_1 \phi (e - e_1)^2 + \frac{1}{2} \left(\sigma - \sigma_a \phi\right) \left(\nabla e\right)^2 + \frac{1}{2} \kappa \left(\nabla^2 e - c_0\right)^2 \\ &+ \frac{k_B T}{a} \left[\phi \ln \phi + (1 - \phi) \ln\left(1 - \phi\right)\right] - h_\phi \phi + \frac{1}{2} D_\phi (\nabla \phi)^2 \end{aligned} \right\}. \tag{S77}$$

We consider the following gradient-descent dynamics:

$$\begin{aligned} \frac{\partial e}{\partial t} &= -k_0 \left(e - e_0\right) - k_1 \phi \left(e - e_1\right) - \sigma_a \nabla\phi \cdot \nabla e + \left(\sigma - \sigma_a \phi\right) \nabla^2 e - \kappa \nabla^4 e + \eta\left(\boldsymbol{x}, t\right), \\ \frac{\partial \phi}{\partial t} &= -\frac{1}{2} k_1 (e - e_1)^2 - \frac{k_B T}{a} \ln\left(\frac{\phi}{1 - \phi}\right) + \frac{1}{2} \sigma_a (\nabla e)^2 + h_\phi + D_\phi \nabla^2 \phi, \end{aligned} \tag{S78}$$

where $\eta\left(\boldsymbol{x}, t\right)$ is the fluctuation, assumed to be Gaussian white noise, satisfying $\langle \eta\left(\boldsymbol{x}, t\right) \rangle = 0$ and $\langle \eta\left(\boldsymbol{x}, t\right) \eta\left(\boldsymbol{x}', t'\right) \rangle = \Lambda^2 \delta\left(\boldsymbol{x} - \boldsymbol{x}'\right) \delta\left(t - t'\right)$ with $\Lambda$ being the noise intensity.

*Simulation results* – We next perform simulations for the governing equation (S78). Here, we set $k_1 = 4k_0$ and $e_1 = \pm 0.2 e_0$. We found that either $e_1 = 0.2 e_0$ and $e_1 = -0.2 e_0$ lead to the appearance of clusters that merge into long linear structures or cross-linked networks upon increasing $\sigma_a$ (Fig. S8).

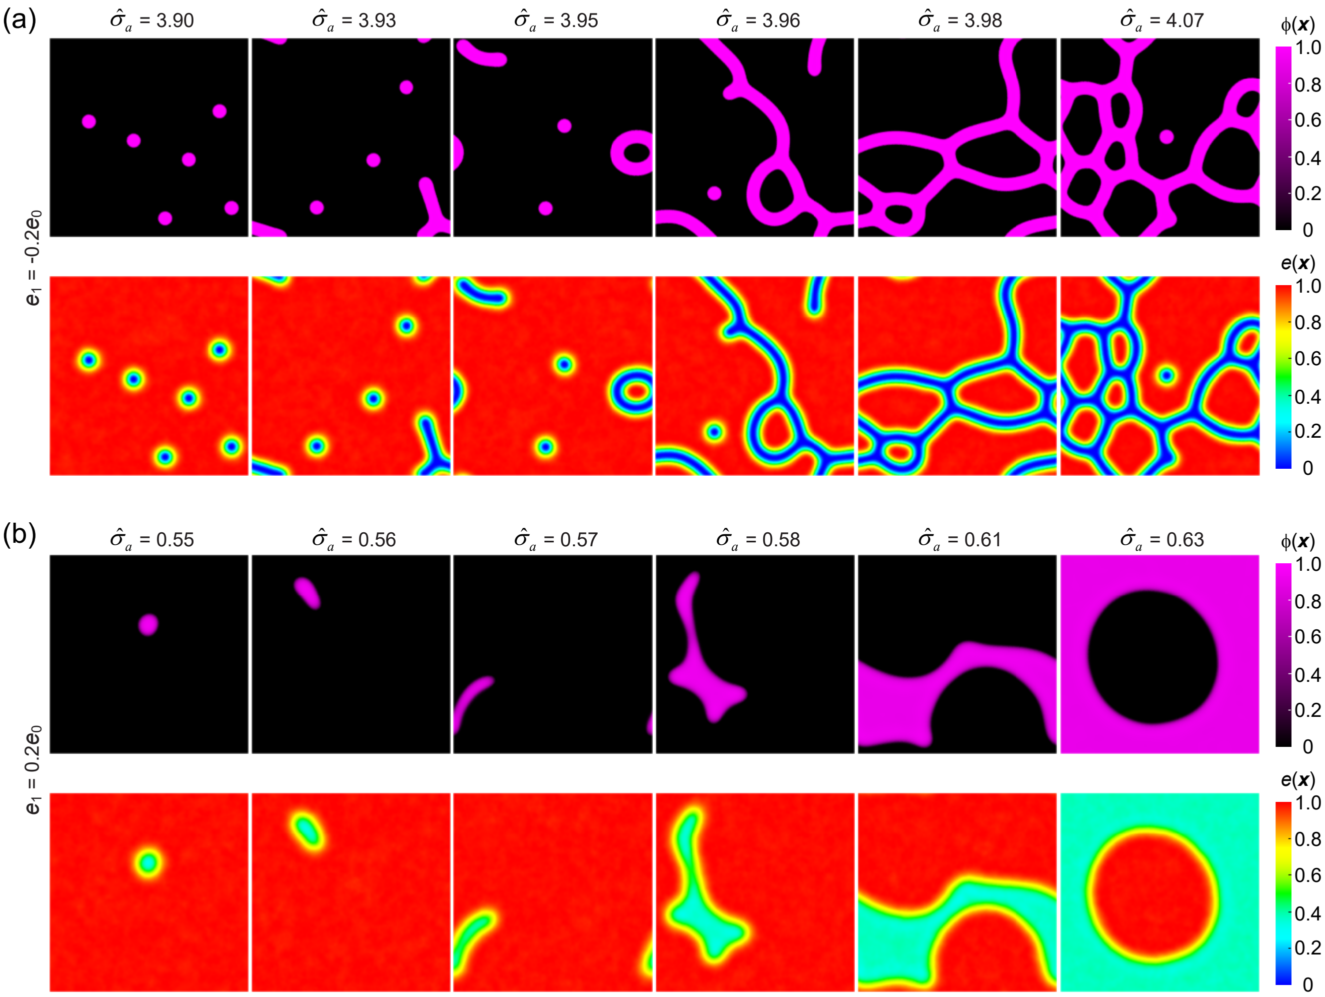


FIG. S8. A $\phi$-dependent membrane-substrate stiffness $k(\phi)$ (Eq. (S76)) leads to similar phases upon increasing the rescaled intensity of protein tilt, $\hat{\sigma}_a = (\sigma_a - \sigma)/\sqrt{k_0\kappa}$. (a) The case of $e_1 = -0.2e_0 < 0$. Top: the $\phi(\boldsymbol{x})$ field; bottom: the $e(\boldsymbol{x})$ field. Simulation box size $L \times L$ with $L = 16e_0 = 1280$ nm. (b) The case of $e_1 = 0.2e_0 > 0$. Top: the $\phi(\boldsymbol{x})$ field; bottom: the $e(\boldsymbol{x})$ field. Simulation box size $L \times L$ with $L = 16e_0 = 1280$ nm. Parameters: $k_1 = 4k_0$, $\hat{h}_\phi = h_\phi/(k_0 e_0^2) = 0.4$. See Table S1 for other parameter values.

## V. SUPPLEMENTAL MOVIES

**Movie S1. $h_\phi$-induced first-order transition** In the low temperature regime ($T < T^{\text{cr}}$), the membrane-protein-substrate system undergoes a first-order transition upon increasing the chemical potential, $h_\phi$, from $h_\phi < h_\phi^{\text{cr},1}$, through $h_\phi^{\text{cr},1} < h_\phi < h_\phi^{\text{cr},3}$, $h_\phi = h_\phi^{\text{cr},3}$, and $h_\phi^{\text{cr},3} < h_\phi < h_\phi^{\text{cr},2}$, to $h_\phi > h_\phi^{\text{cr},2}$. Here, $F_{\text{min}} = \min_{\phi\in(0,1)} \{F(\phi)\}$. The color bar represents the value of $h_\phi$; the circular purple dots indicate local mimina or local maxima.

**Movie S2. Temperature-induced phase transition** The membrane-protein-substrate system transitions from a dilute state $\phi \approx 0$ (for $h_\phi < h_\phi^{\text{cr},3}$ shown here), or a dense state $\phi \approx 1$ (correspondingly for $h_\phi > h_\phi^{\text{cr},3}$), to a disordered state ($\phi \approx 1/2$) upon increasing the temperature $T$ to beyond a critical value, $T^{\text{cr}}$. Here, $F_{\text{min}} = \min_{\phi\in(0,1)} \{F(\phi)\}$. The color bar represents the value of $T$; the circular purple dots indicate local mimina or local maxima.


[1] R. Changede, X. Xu, F. Margadant, and M. Sheetz, Developmental Cell **35**, 614 (2015).
[2] R. Changede, H. Cai, S. J. Wind, and M. P. Sheetz, Nature Materials **18**, 1366 (2019).
[3] J. Swift and P. C. Hohenberg, Physical Review A **15**, 319 (1977).
[4] R. B. Hoyle, *Pattern formation: An introduction to methods* (Cambridge University Press, 2006).
[5] T. M. Inc., Matlab version: 9.13.0 (r2022b) (2022).
[6] G. Popescu, T. Ikeda, K. Goda, C. A. Best-Popescu, M. Laposata, S. Manley, R. R. Dasari, K. Badizadegan, and M. S. Feld, Physical Review Letters **97**, 218101 (2006).
[7] M. M. Kozlov and L. V. Chernomordik, Current Opinion in Structural Biology **33**, 61 (2015).
[8] I. Raote, M. Chabanon, N. Walani, M. Arroyo, M. F. Garcia-Parajo, V. Malhotra, and F. Campelo, eLife **9**, e59426 (2020).
[9] T. Bihr, U. Seifert, and A.-S. Smith, Physical Review Letters **109**, 258101 (2012).
[10] A.-S. Smith, K. Sengupta, S. Goennenwein, U. Seifert, and E. Sackmann, Proceedings of the National Academy of Sciences of the United States of America **105**, 6906 (2008).
[11] T. Bihr, U. Seifert, and A.-S. Smith, New Journal of Physics **17**, 083016 (2015).
[12] T. R. Weikl, Annual Review of Physical Chemistry **69**, 521 (2018).
[13] J. Steinkühler, E. Sezgin, I. Urbančič, C. Eggeling, and R. Dimova, Communications Biology **2**, 337 (2019).
[14] X.-P. Xu, E. Kim, M. Swift, J. Smith, N. Volkmann, and D. Hanein, Biophysical Journal **110**, 798 (2016).
